# Supplementary material for: Interpreting Low-level Vision Models with Causal Effect Maps
Source: arXiv:2407.19789 source file (2025-03-31)
Supplement: Supplementary file 1 [file Appendix.tex]

\section{Appendix}

\subsection{Additional information of CEM}
\label{A:1}

To demonstrate that averaging multiple times to take the expectation is feasible, we conducted experiments on multiple SR models on different patches of diverse images. 
It is found that regardless of the model $\mathcal{F}$, patch $p_i$ and image $I$, the $\phi_\mathcal{F}[p_i]$ can converge to a stable value as the number of interventions increases as shown in Fig. \ref{fig:converge}.
Also, the effectiveness of the probability density $\mathcal{D}$ should be analyzed.
$\mathcal{D}$ is obtained from image gradients.
The image gradient of image $I$ is calculated as:
\begin{equation}
\small
    G = \sqrt{\Sigma(I(x,:)-I(x-1,:))^2+\Sigma(I(:,y)-I(:,y-1))^2},
\end{equation}
where $x$ and $y$ is the index of column and row.
It should be noted that the manner of calculating the gradient does not need to be consistent with the above equation, as long as it can be used as a measure of variation in the content of the image.
We also try to sample the intervention patches using the uniform probability.
Additionally, the number of interventions in the fine stage of CEM calculation is a hyperparameter, which can be discussed.
The proportion of inference times and similarity scores for different intervention strategies compared to the proposed setting are recorded in Tab. \ref{tab:A1}.

\begin{table}[h]
\label{tab:A1}
    \centering\setlength{\tabcolsep}{6pt}
    % \hspace{-4mm}
    % \small
    \begin{tabular}{lcc}
                \Xhline{1.2pt}
                Interventions & Inferences & Similarity Score \\
                \Xhline{1.2pt}
                3C10F&1.3\%& 65,32\% \\
                3C30F&2.8\% & 78.68\% \\
                3C50F-U& 4.9\%&77.72\% \\
                1C50F& 2.9\%&75.86\% \\
                3C50F (ours)& 4.9\% &82.62\% \\

                \Xhline{1.2pt}
  \end{tabular}
    % \vspace{-3mm}
    \caption{The proportion of inference times and similarity scores for different intervention strategies compared to the original method. C and F denote the inference times used in the coarse stage and fine stage, respectively. U represents sampling with uniform probability.}
    % \vspace{-4mm}
\end{table}

\subsection{Model Collection}

Models in the experiments encompass basic CNN and residual networks: SRCNN \cite{SRCNN}, EDSR \cite{EDSR}, CARN \cite{CARN}, SRDenseNet \cite{SRDenseNet}, SRResNet \cite{SRResNet}, DnCNN \cite{DnCNN}, FFDNet \cite{FFDNet}, SADNet \cite{SADNet}, PReNet \cite{PReNet}, and HINet \cite{HINet};
attention mechanisms with global receptive fields: DRLN \cite{DRLN}, RNAN \cite{RNAN}, RCAN \cite{RCAN}, SAN \cite{SAN}, and MPRNet \cite{MPRNet}. 
Transformer-based networks:  SwinIR \cite{SWinIR}, SCUNet \cite{SCUNet}, HAT \cite{HAT}, and X-Restormer \cite{XRestormer}.

\subsection{More CEM results of LV models}
More CEM results of super-resolution (SR), denoising (DN), and draining (DR) models are presented in Fig.\ref{fig:Exp1}, Fig.\ref{fig:Exp2}, and Fig.\ref{fig:Exp3} respectively.

\input{figs/converge}

% \begin{figure*}[t] 
% \centering
%     \includegraphics[width=0.9\linewidth]{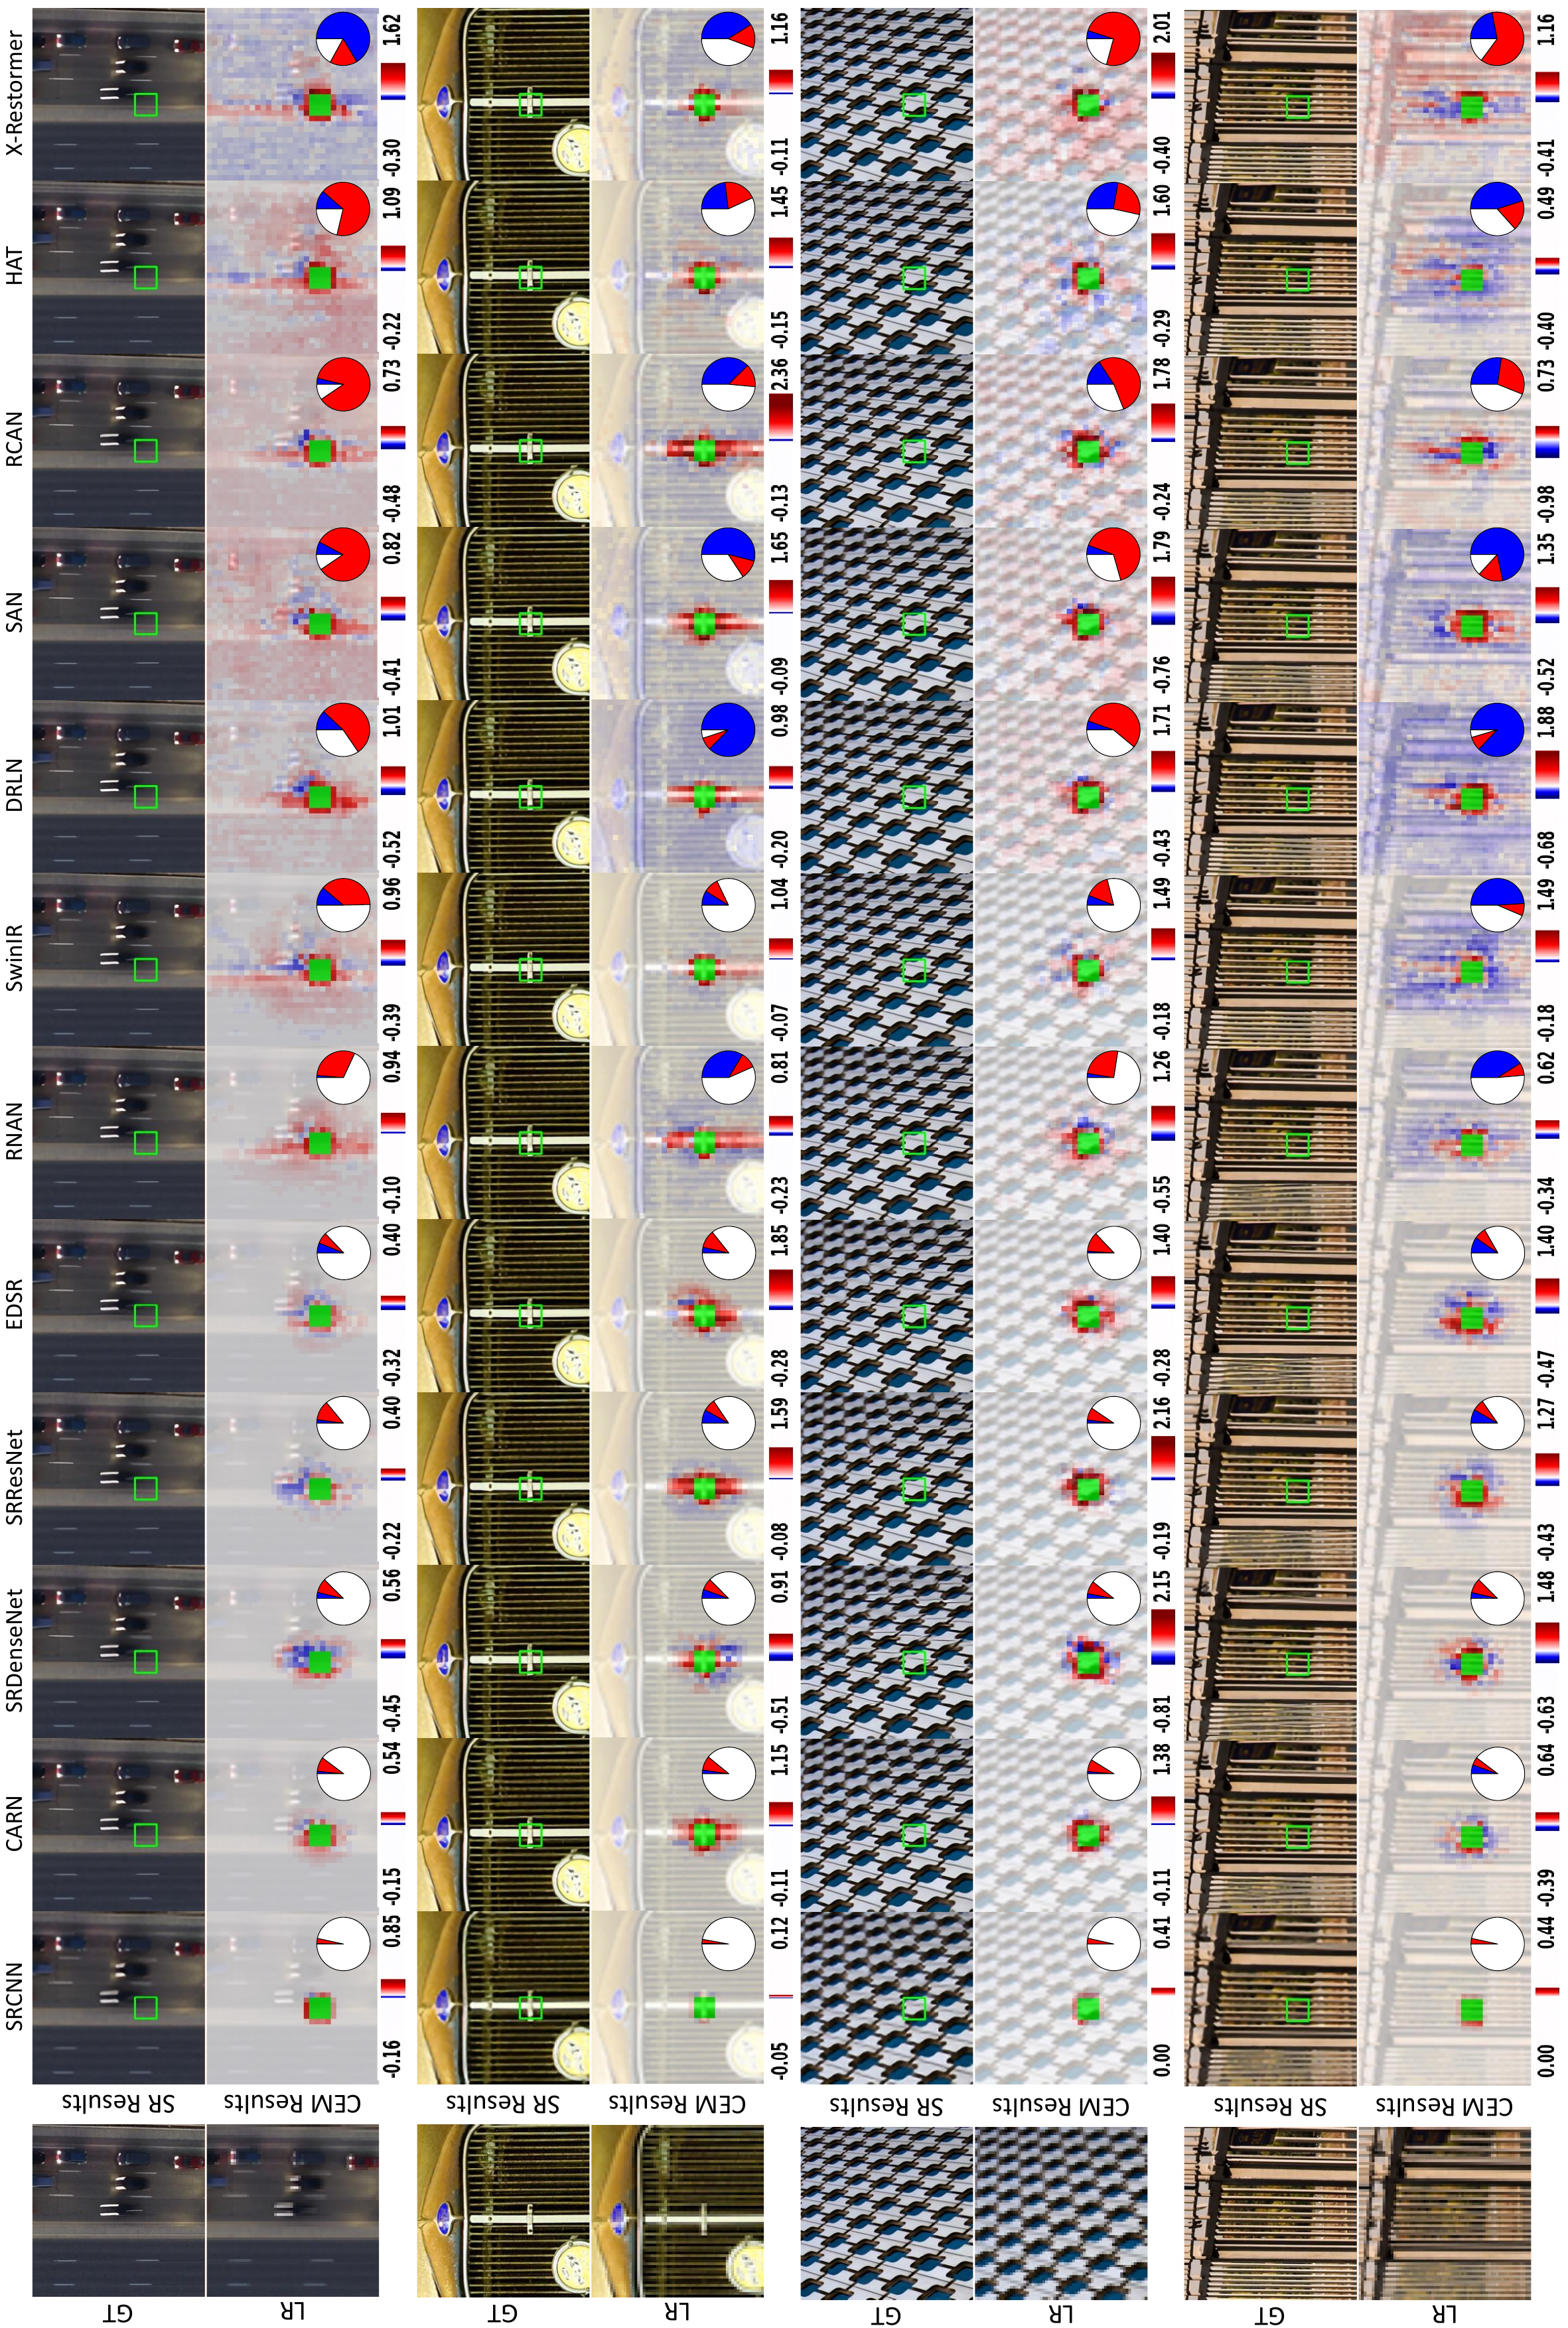}
%     \caption{More CEM results of SR networks.}
%     \label{fig:Exp1}
% \end{figure*}

\begin{figure*}[htbp]
  \centering
  \rotatebox{90}{%
    \begin{minipage}{\textheight}
    \centering
\includegraphics[width=1\linewidth]{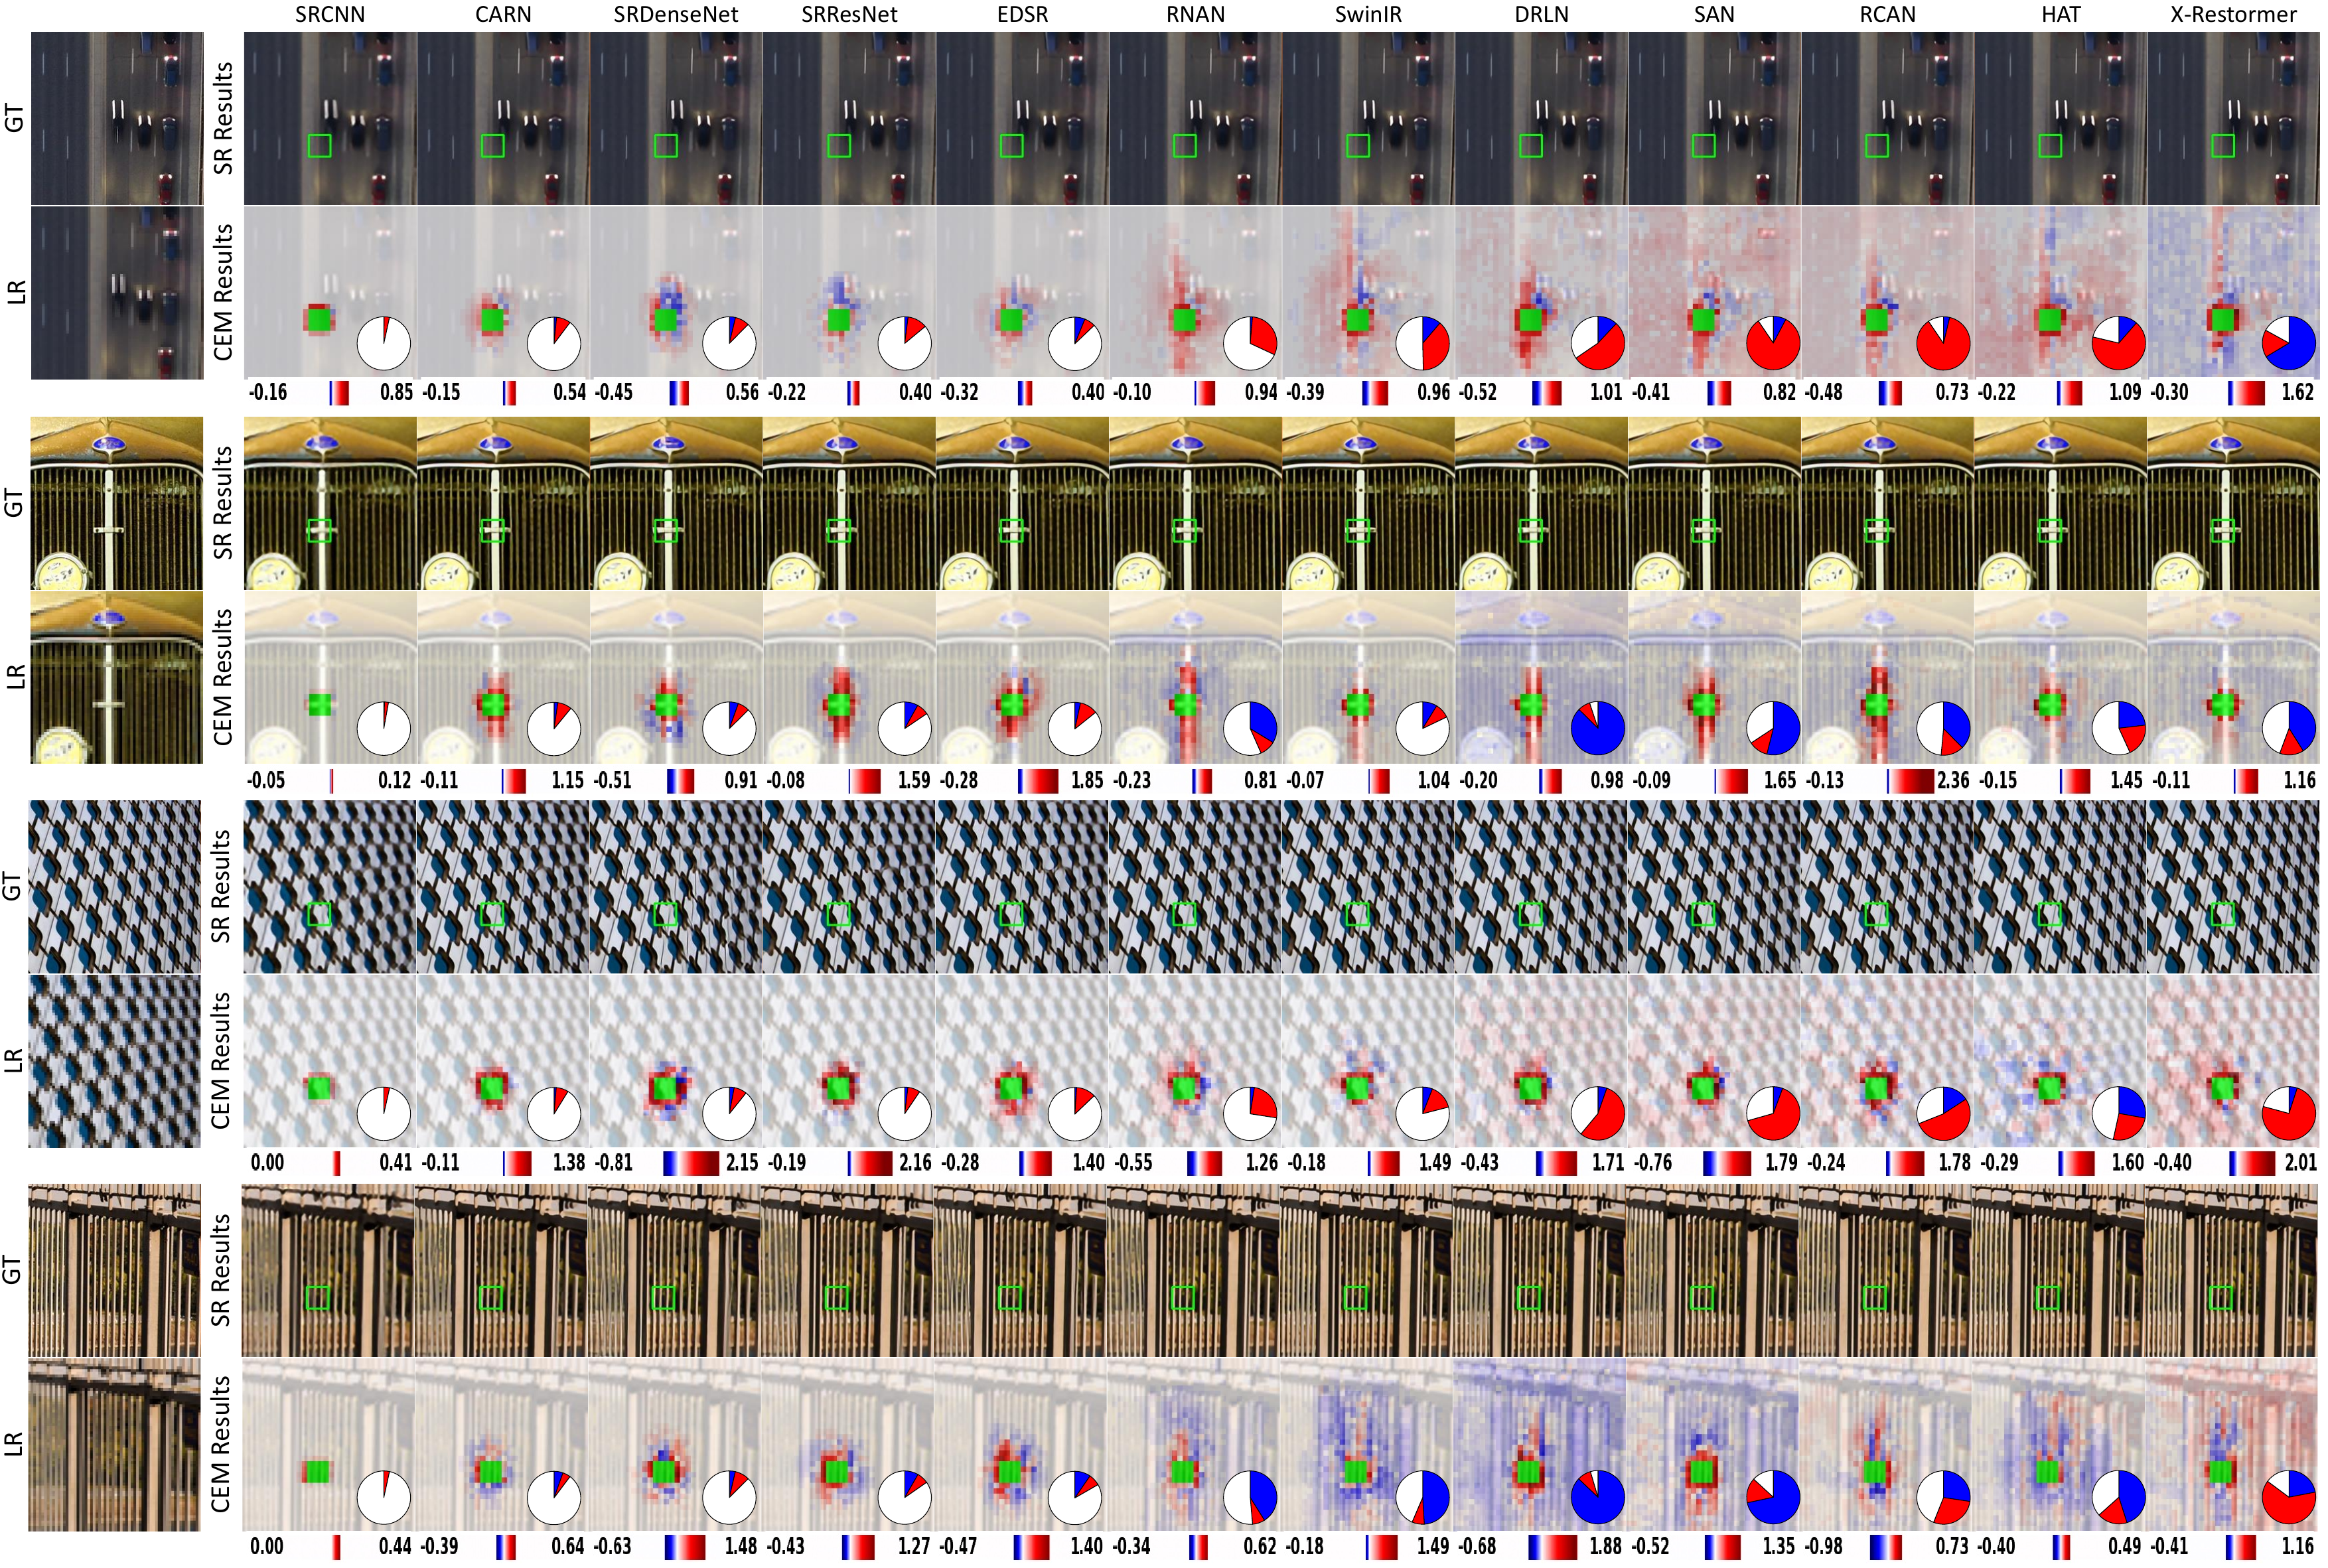}
    \caption{More CEM results of SR networks.}
    \label{fig:Exp1}
    \end{minipage}%
  }
\end{figure*}

\newpage

% \begin{figure}[htbp]
%   \centering
%   \rotatebox{90}{%
%     \begin{minipage}{\textheight}
%     \centering
% \includegraphics[width=1\linewidth]{figs/sources/more_result_SR_modified.pdf}
%     \caption{More CEM results of SR networks.}
%     \label{fig:Exp1}
%     \end{minipage}%
%   }
% \end{figure}

\begin{figure*}[htbp]
  \centering
  \rotatebox{90}{%
    \begin{minipage}{\textheight}
    \centering
    \includegraphics[width=0.85\linewidth]{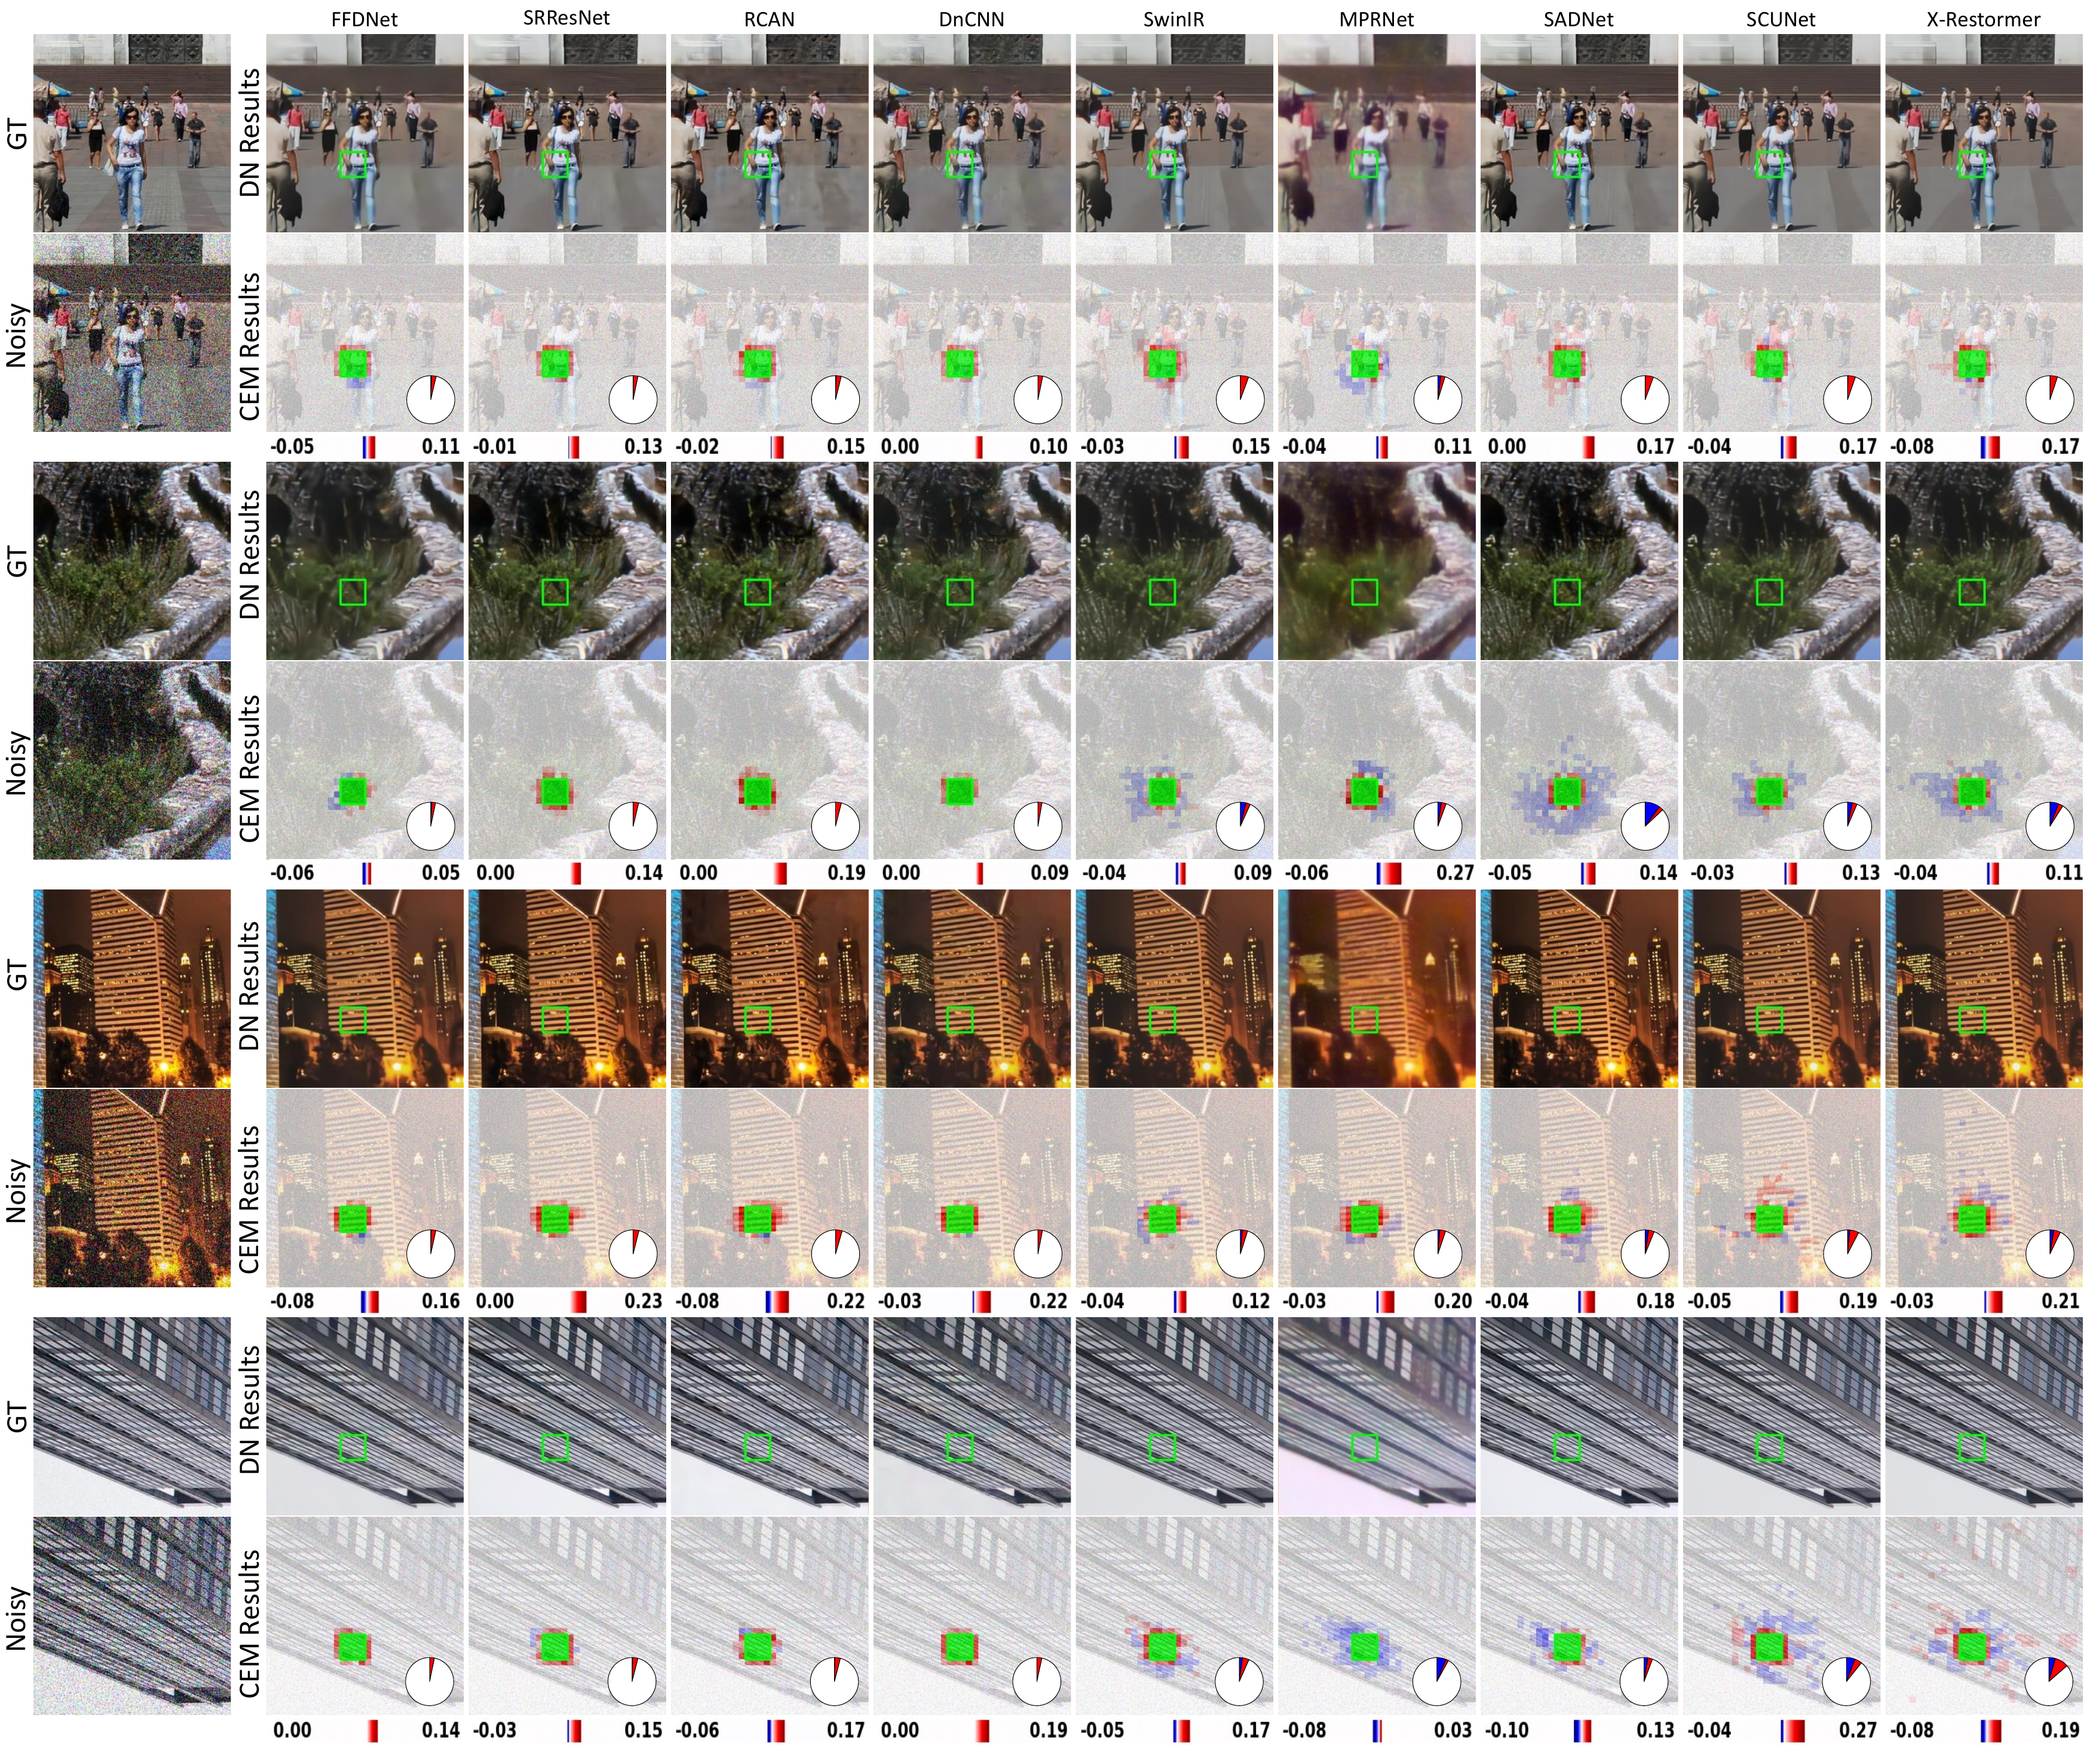}
    \caption{More CEM results of DN networks.}
    \label{fig:Exp2}
    \end{minipage}%
  }
\end{figure*}
\newpage
\begin{figure*}[htbp]
  \centering
  \rotatebox{90}{%
    \begin{minipage}{\textheight}
    \centering
    \includegraphics[width=0.89\linewidth]{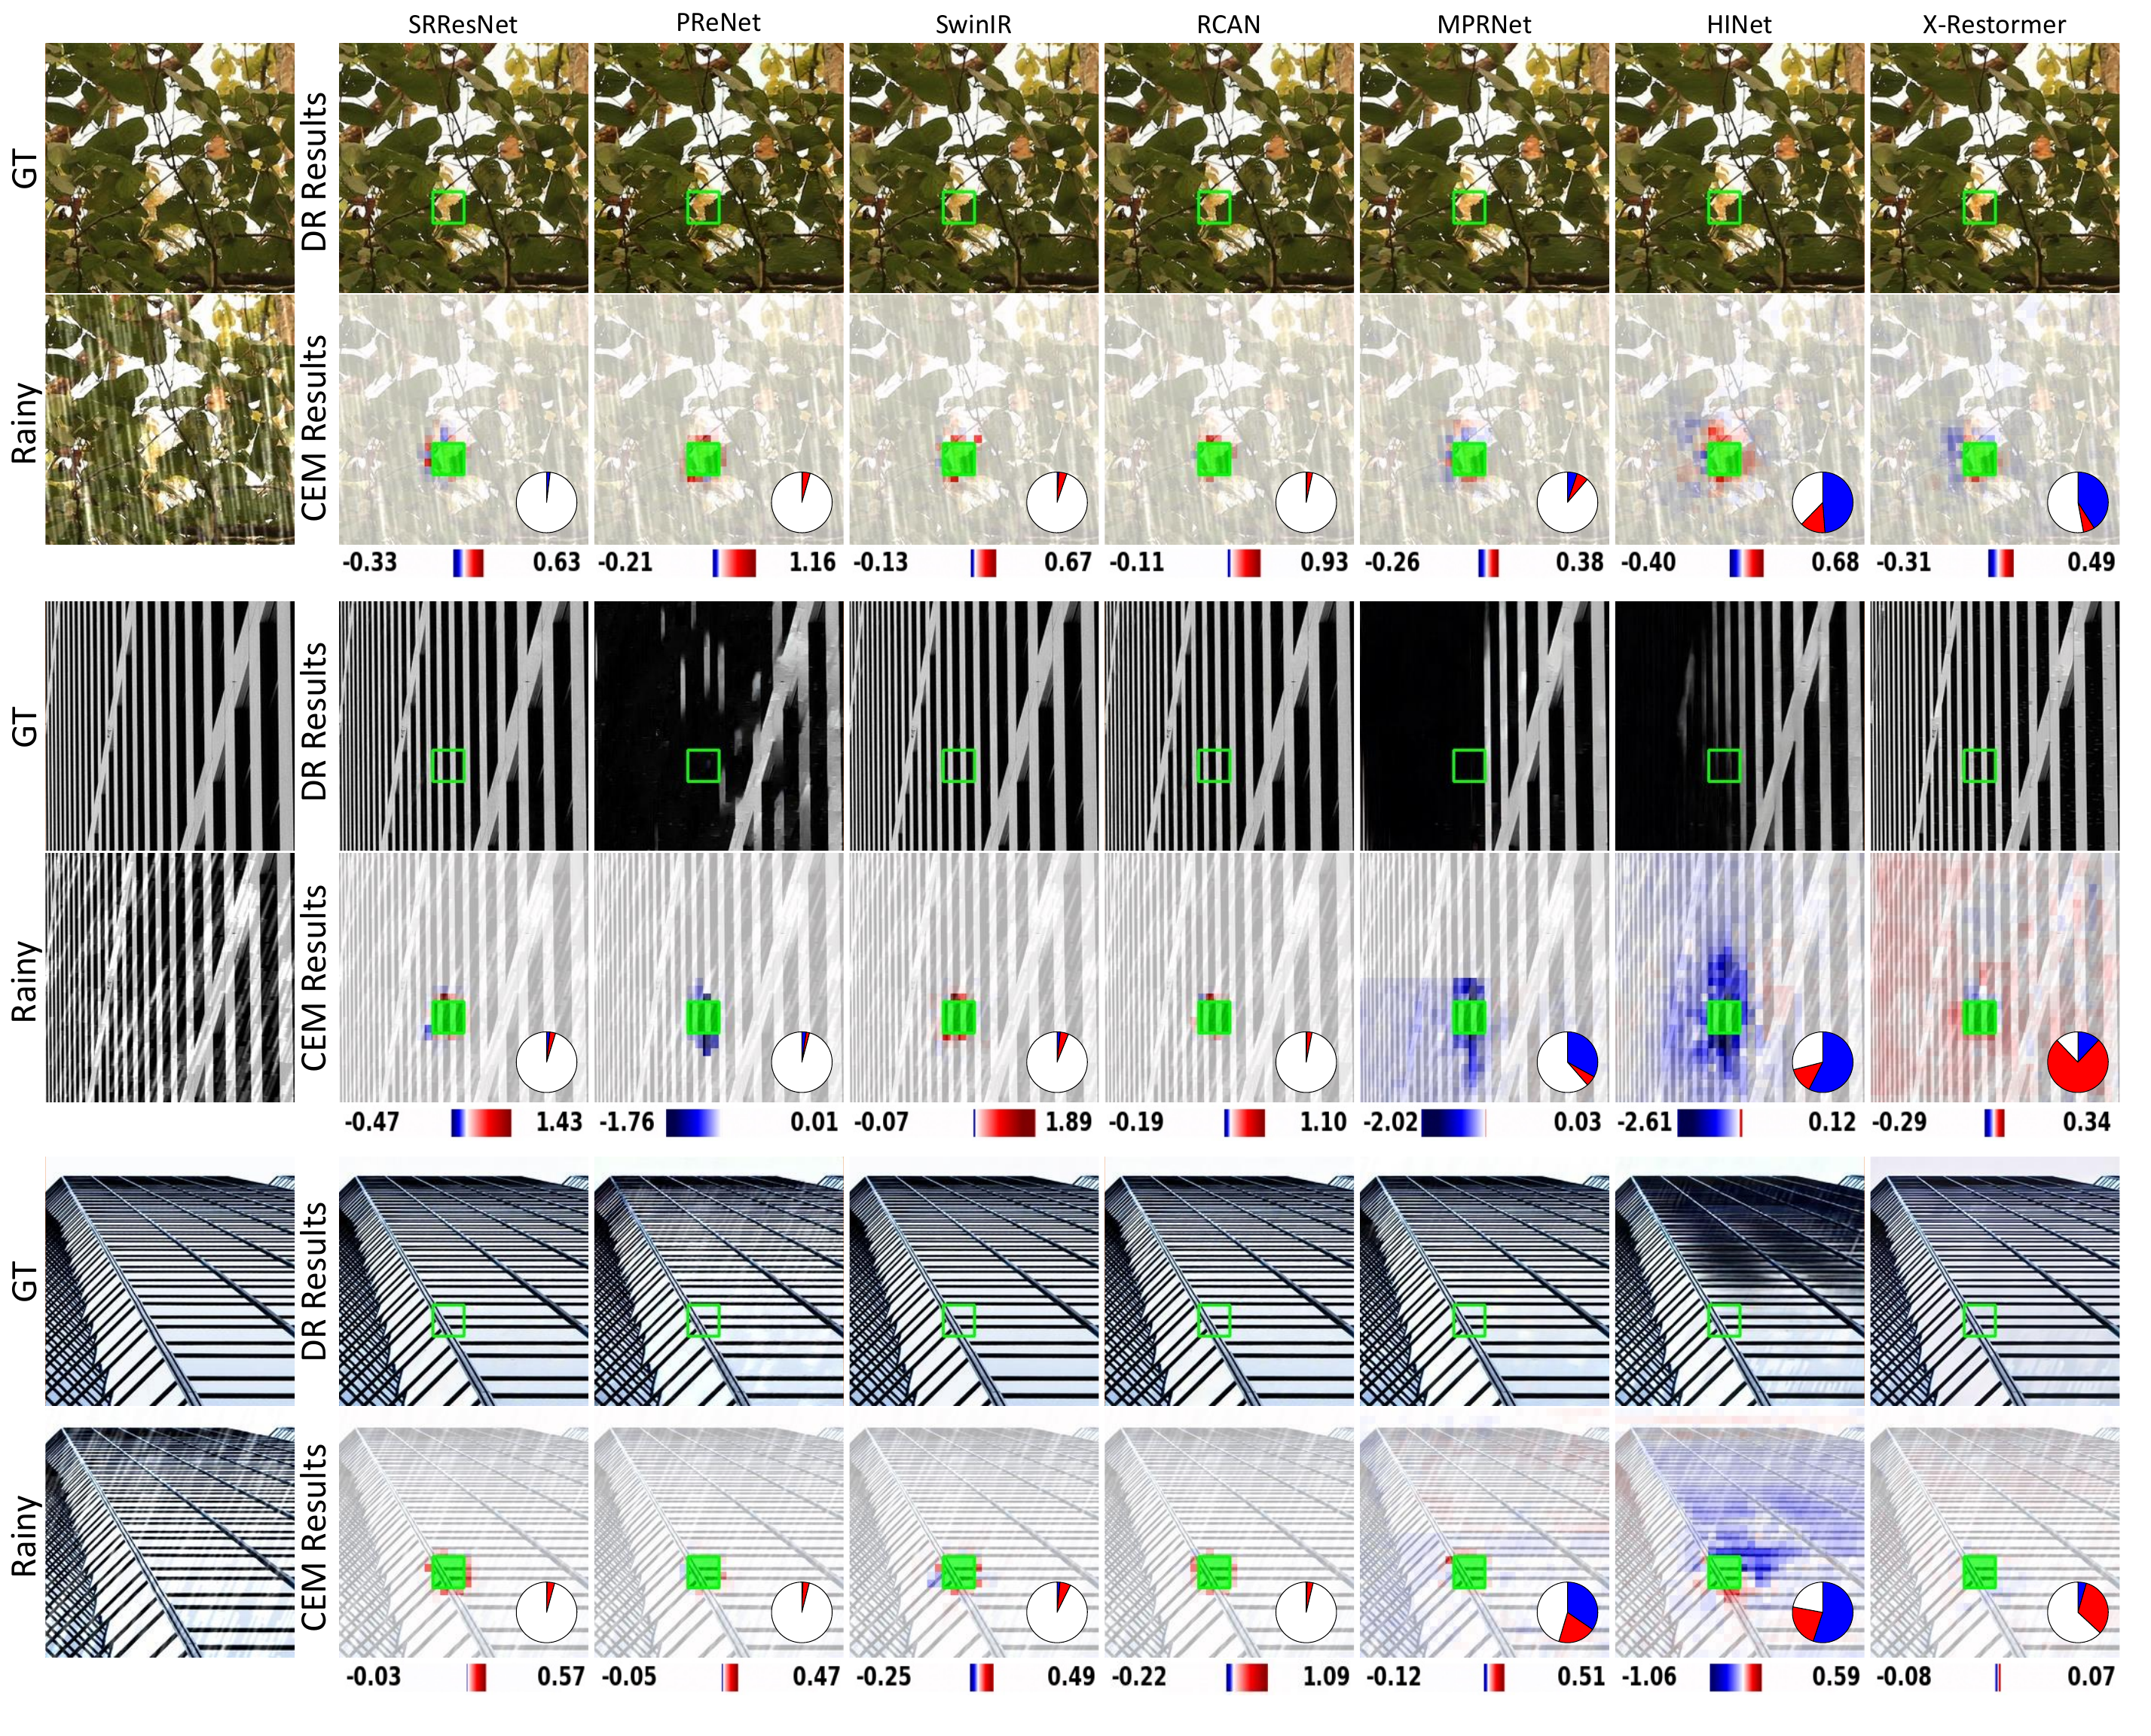}
    \caption{More CEM results of DR networks.}
    \label{fig:Exp3}
    \end{minipage}%
  }
\end{figure*}
